# Supplementary material for: TeraHAC: Hierarchical Agglomerative Clustering of Trillion-Edge Graphs
Source: arXiv:2308.03578 source file (2024-06-11)
Supplement: Supplementary file 1 [file appendix.tex]

\ifx\confversion\undefined
\balance
\clearpage
\appendix
\input{appendix-proofs}
In this section we provide additional experimental figures and
results that we did not have sufficient space to include in the
main paper.

\subsection{Tuning $\epsilon$ with no thresholding}

\begin{figure*}
%\vspace{1em}
\begin{minipage}{.49\textwidth}
\hspace{-1em}
    \includegraphics[width=\textwidth]{figures/iris-ARI.pdf}
\end{minipage}%\hfill
%\hspace{1em}
\begin{minipage}{0.49\textwidth}
  \includegraphics[width=\textwidth]{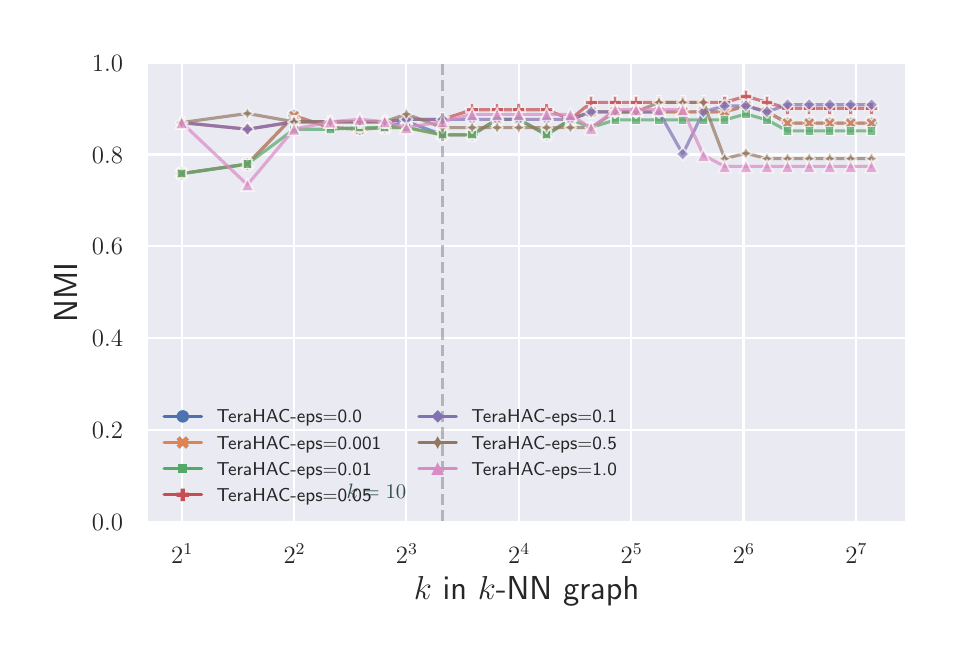}
\end{minipage}\\
\begin{minipage}[t]{.49\textwidth}
  \caption{\small Adjusted Rand-Index (ARI) of clusterings computed by
  \parhac{} for varying $\epsilon$ on Iris  versus the $k$
  used in similarity graph construction.
\label{fig:iris-ARI}}
\end{minipage}\hfill
\begin{minipage}[t]{.49\textwidth}
  \caption{\small Normalized Mutual Information (NMI) of clusterings
  computed by \parhac{} for varying $\epsilon$ on Iris 
  versus the $k$ used in similarity graph construction.
\label{fig:iris-NMI}}
\end{minipage}
\end{figure*}
\begin{figure*}
%\vspace{1em}
\begin{minipage}{.49\textwidth}
\hspace{-1em}
    \includegraphics[width=\textwidth]{figures/iris-Purity.pdf}
\end{minipage}%\hfill
%\hspace{1em}
\begin{minipage}{0.49\textwidth}
  \includegraphics[width=\textwidth]{figures/iris-Dasgupta.pdf}
\end{minipage}\\
\begin{minipage}[t]{.49\textwidth}
  \caption{\small Dendrogram Purity (Purity) of clusterings computed by
  \parhac{} for varying $\epsilon$ on Iris  versus the $k$
  used in similarity graph construction.
\label{fig:iris-Purity}}
\end{minipage}\hfill
\begin{minipage}[t]{.49\textwidth}
  \caption{\small Dasgupta Cost (Dasgupta) of clusterings
  computed by \parhac{} for varying $\epsilon$ on Iris 
  versus the $k$ used in similarity graph construction.
\label{fig:iris-Dasgupta}}
\end{minipage}
\end{figure*}

\fi
